# Supplementary material for: Learning to Predict Usage Options of Product Reviews with LLM-Generated Labels
Source: arXiv:2410.12470 source file (2024-10-16)
Supplement: Supplementary file 1 [file prompt_selection.tex]

\begin{figure}
\resizebox{\textwidth}{!}{
\begin{tabular}{llcccc}
\caption{Performance of LLM prompts on test dataset $\mathcal A$.}
\textbf{Model} & \textbf{Prompt} & \textbf{Harmonic Score} & \textbf{Positives Score} & \textbf{Negatives Score} & \textbf{Accuracy} \\
\hline\\
Llama 2 7B & CoT 6-shot & \pmb{0.45} & 0.48 & 0.42 & 0.69 \\
Llama 2 7B & CoT 2-shot & 0.38 & 0.52 & 0.30 & 0.64 \\
Llama 2 7B & 6-shot & 0.30 & 0.43 & 0.23 & 0.60 \\
Llama 2 7B & 2-shot & 0.28 & 0.38 & 0.22 & 0.61 \\
\hline
Llama 2 13B & CoT 6-shot & 0.48 & 0.53 & 0.43 & 0.71 \\
Llama 2 13B & CoT 2-shot & 0.57 & 0.54 & 0.61 & 0.77 \\
Llama 2 13B & 6-shot & 0.54 & 0.38 & 0.91 & 0.78 \\
Llama 2 13B & 2-shot & \pmb{0.63} & 0.51 & 0.82 & 0.87 \\
\hline
Llama 2 70B & CoT 6-shot & 0.25 & 0.60 & 0.16 & 0.58 \\
Llama 2 70B & CoT 2-shot & \pmb{0.50} & 0.60 & 0.43 & 0.71 \\
Llama 2 70B & 6-shot & 0.33 & 0.47 & 0.25 & 0.62 \\
Llama 2 70B & 2-shot & 0.47 & 0.56 & 0.40 & 0.70 \\
\hline
GPT 3.5 Turbo & CoT 6-shot & 0.68 & 0.63 & 0.75 & 0.84 \\
GPT 3.5 Turbo & CoT 2-shot & 0.74 & 0.69 & 0.81 & 0.88 \\
GPT 3.5 Turbo & 6-shot & 0.77 & 0.69 & 0.86 & 0.92 \\
GPT 3.5 Turbo & 2-shot & \pmb{0.79} & 0.68 & 0.94 & 0.90 \\
\hline
GPT 4 & CoT 6-shot & 0.72 & 0.72 & 0.72 & 0.85 \\
GPT 4 & CoT 2-shot & 0.69 & 0.70 & 0.67 & 0.83 \\
GPT 4 & 6-shot & \pmb{0.81} & 0.76 & 0.88 & 0.92 \\
GPT 4 & 2-shot & 0.78 & 0.75 & 0.82 & 0.90 \\
\end{tabular}}

\end{figure}
